# Supplementary material for: Ranking Regularization for Critical Rare Classes: Minimizing False Positives at a High True Positive Rate
Source: arXiv:2304.00049 source file (2023-03-31)
Supplement: Supplementary file 1 [file supp.tex]

% CVPR 2023 Paper Template
% based on the CVPR template provided by Ming-Ming Cheng (https://github.com/MCG-NKU/CVPR_Template)
% modified and extended by Stefan Roth (stefan.roth@NOSPAMtu-darmstadt.de)

\documentclass[10pt,twocolumn,letterpaper]{article}

%%%%%%%%% PAPER TYPE  - PLEASE UPDATE FOR FINAL VERSION
%\usepackage[review]{cvpr}      % To produce the REVIEW version
\usepackage{cvpr}              % To produce the CAMERA-READY version
%\usepackage[pagenumbers]{cvpr} % To force page numbers, e.g. for an arXiv version

% Include other packages here, before hyperref.
\usepackage{graphicx}
\usepackage{amsmath}
\usepackage{amssymb}
\usepackage{booktabs}
\usepackage[dvipsnames]{xcolor}
\usepackage{tikz,pgfplots}
    \usepgfplotslibrary{groupplots}
\usepackage{graphicx}
\usepackage{multirow}

% Kiarash imports:
\usepackage{bm}
\usepackage{bbm}

% Kiarash commands:

% \setlength{\abovedisplayskip}{3pt}
% \setlength{\belowdisplayskip}{3pt}
% \setlength{\textfloatsep}{3pt}
% \setlength{\parindent}{15pt}
%\setlength{\parskip}{3pt}

\definecolor{lb}{RGB}{44, 139, 183}

% It is strongly recommended to use hyperref, especially for the review version.
% hyperref with option pagebackref eases the reviewers' job.
% Please disable hyperref *only* if you encounter grave issues, e.g. with the
% file validation for the camera-ready version.
%
% If you comment hyperref and then uncomment it, you should delete
% ReviewTempalte.aux before re-running LaTeX.
% (Or just hit 'q' on the first LaTeX run, let it finish, and you
%  should be clear).
\usepackage[pagebackref,breaklinks,colorlinks]{hyperref}

% Support for easy cross-referencing
\usepackage[capitalize]{cleveref}
\crefname{section}{Sec.}{Secs.}
\Crefname{section}{Section}{Sections}
\Crefname{table}{Table}{Tables}
\crefname{table}{Tab.}{Tabs.}

%%%%%%%%% PAPER ID  - PLEASE UPDATE
 % *** Enter the CVPR Paper ID here

\usepackage{xcolor,colortbl}

\definecolor{Gray}{gray}{0.85}
\definecolor{LightCyan}{rgb}{0.88,1,1}

\newcolumntype{a}{>{\columncolor{Gray}}c}
\newcolumntype{b}{>{\columncolor{white}}c}

\begin{document}

%%%%%%%%% TITLE - PLEASE UPDATE
% \title{
% Supplemental Material: Ranking Regularization for Critical Rare Classes: Minimizing False Positives at a High True Positive Rate}

% \author{Kiarash Mohammadi$^{1,2}$ \quad He Zhao$^1$ \quad Mengyao Zhai$^1$ \quad Frederick Tung$^1$\\
% $^{1}$Borealis AI \quad $^{2}$ Mila, Universit{\'e} de Montr{\'e}al\\
% {\tt\small kiarash.mohammadi@mila.quebec, \{he.zhao, mengyao.zhai, frederick.tung\}@borealisai.com}

% }
% \maketitle

%%%%%%%%% ABSTRACT
% \begin{abstract}
% This document provides additional material that is supplemental to our main submission. In particular, we provide
% the experimental results for more skewed imbalanced ratio, namely 1:200, for the imbalanced CIFAR-10 and 100 datasets, as discussed in Section 4.5 of the
% main submission. 
% \end{abstract}

\section*{A. Additional Results}
\input{figures/main_5.tex}
\newpage 
% \section*{B. Additional Results}
\vspace*{0.65em}
\input{figures/main_4.tex}
% \newpage
%%%%%%%%% REFERENCES
{\small
\bibliographystyle{ieee_fullname}
\bibliography{egbib}
}

\end{document}
