# Supplementary material for: Ranking Regularization for Critical Rare Classes: Minimizing False Positives at a High True Positive Rate
Source: arXiv:2304.00049 source file (2023-03-31)
Supplement: Supplementary file 2 [file supp_intro.tex]

In this document, we provide details of missing components, like datasets,
